# Supplementary material for: Fault friction under thermal pressurization during large coseismic-slip Part I: Numerical analyses
Source: arXiv:2205.00314 source file (2022-04-30)
Supplement: Supplementary file 1 [file AppendixE.tex]

%\chapter{Appendix E \label{Appendix E}}
\section{Derivation of the coupled pore fluid pressure diffusion kernel. \label{Appendix E}}
\noindent In this section we derive the coupled pore fluid pressure diffusion kernel for the cases of a bounded domain subjected to a stationary Dirac load and an unbounded domain under a moving Dirac load. Our procedure follows the discussion in \cite{Lee1987} where the same problem was solved for a stationary Dirac thermal load on an unbounded domain.

\subsection{Stationary thermal load, coupled pore fluid pressure Green's kernel for a bounded domain.}

\noindent In the case of the bounded domain we proceed by applying the method of separation of variables and then expanding the solution to a Fourier series. We note here that the coupled system of pressure and temperature diffusion equations have the same form of linear partial differential operators and boundary conditions and therefore their solution belongs to the same space of Sturn-Liouville problems. In essence the two solutions have the same eigenfunctions. In the case of the bounded domain the Temperature diffusion equation has the solution given in \cite{cole2010heat}:
\begin{align}
T(x,t) = \sum_{n=1}^\infty\frac{2}{\text{H} \rho C}\int_0^{t}\int_{-\infty}^\infty g(x^\prime, t^\prime)\exp{\left[-\lambda^2 c_{th}(t-t^\prime)\right]}\sin{\left(\lambda_n x\right)}\sin{\left(\lambda_n x^\prime\right)}dx^\prime dt^\prime,
\end{align} 
\noindent where $\lambda_n$ is the Sturm-Liouvile eigenfunction coefficient, $\lambda_n=\frac{n\pi}{\text{H}}$, $\text{H}$ is the length of the bounded domain. The eigencondition for the homogeneous Dirichlet boundary condtitions are given by:
\begin{align}
\sin\left({\frac{n\pi}{\text{H}}\text{H}}\right)=0,\; \lambda_n=\frac{n\pi}{\text{H}},\; n=1,2,...
\end{align}
\noindent We note here that the homogeneous pressure diffusion partial deifferential equation on the above bounded domain has the same boundary conditions. Therefore, the pore fluid pressure solution can be written with the same eigenfunctions as above. Replacing the pore fluid pressure eigenfunction expansion $\tilde{p}(x,t)=p(x,t)-p_0=\sum_{i=n}^\infty \tilde{p}_n\sin{\frac{n\pi x}{\text{H}}}$ into the coupled pressure diffusion partial differential equation,
\begin{align}
&\frac{\partial \tilde{p}(x,t)}{\partial t}-c_{hy}\frac{\partial^2 \tilde{p}(x,t)}{\partial x^2}=\Lambda\frac{\partial T(x,t)}{\partial t},\nonumber\\
&\tilde{p}(x,0)=0, \nonumber\\
&\tilde{p}(0,t)=\tilde{p}(\text{H},t)=0,
\end{align}
\noindent we obtain:
\begin{align}
\sum_{n=1}^\infty\frac{\partial \tilde{p}_n(t)}{\partial t}\sin{\lambda_n x}+c_{hy}\sum_{n=1}^\infty \lambda^2_n\tilde{p}_n(t)\sin{\lambda_n x}= \frac{2 \Lambda}{\text{H} \rho C}\sum_{n=1}^\infty\sin{\lambda_n x} \frac{\partial T_n{(t)}}{\partial t}&,\\
\intertext{where $T_n(t)$ is given as:}
T_n(t)=\int_0^t\int_{-\infty}^\infty g(x^\prime, t^\prime)\exp{\left[-\lambda_n^2 c_{th}(t-t^\prime)\right]}\sin{\lambda_n x^\prime}dx^\prime dt^\prime. \nonumber
\end{align}
\noindent Isolating each eigenfunction $\sin{\lambda_n x}$ we arrive at the following first order linear differential equations involving the unknown coefficient $\tilde{p}_n(t)$ and the loading coefficient $T_n(t)$ for each particular component of the solution series expansion.
\begin{align}
\frac{\partial \tilde{p}_n(t)}{\partial t}+c_{hy} \lambda^2_n\tilde{p}_n(t)=& \frac{2 \Lambda}{\text{H} \rho C}\frac{\partial T_n(t)}{\partial t},\;t\geq 0. 
\end{align}
\noindent Applying the Laplace transformation in the field of time:
\begin{align}
&s\tilde{P}_n(s)+c_{hy} \lambda^2_n\tilde{P}_n(s)=\frac{2 \Lambda}{\text{H} \rho C}\frac{s}{s+\lambda^2_n c_{th}}\int_{-\infty}^\infty G(x^\prime, s)\sin{\lambda_n x^\prime}dx^\prime .\\
&\tilde{P}_n(s)=\frac{2 \Lambda}{\text{H} \rho C}\frac{s}{(s+\lambda^2_n c_{th})(s+\lambda^2_n c_{hy})}\int_{-\infty}^\infty G(x^\prime, s)\sin{\lambda_n x^\prime}dx^\prime
\end{align}
\noindent Applying the inverse of the Laplace transform gives us:
\begin{align}
\tilde{p}_n(x,t) = \frac{2 \Lambda}{\text{H} \rho C }\int_0^t\int_{-\infty}^{\infty}g(x^\prime,t^\prime)\frac{c_{hy} \exp{\left[-\lambda^2_nc_{hy}(t-t^\prime)\right]}-c_{th} \exp{\left[-\lambda^2_nc_{th}(t-t^\prime)\right]}}{c_{hy}-c_{th}}\sin{\lambda_n x^\prime}dx^\prime dt^\prime
\end{align} 
\noindent Finally, in the series expansion $\tilde{p}(x,t)=\sum_{n=1}^\infty \tilde{p}_n(t)\sin{\lambda_n x}$ we move the summation under the integral sign and we obtain:
\begin{align}
\begin{aligned}
\tilde{p}(x,t) = \frac{2 \Lambda}{\text{H} \rho C }\int_0^t\int_{-\infty}^{\infty}&g(x^\prime,t^\prime)\\
&\sum_{n=1}^\infty\frac{c_{hy} \exp{\left[-\lambda^2_nc_{hy}(t-t^\prime)\right]}-c_{th} \exp{\left[-\lambda^2_nc_{th}(t-t^\prime)\right]}}{c_{hy}-c_{th}}\sin{\lambda_n x}\sin{\lambda_n x^\prime}dx^\prime dt^\prime
\end{aligned} \label{app E: eq: bounded Green's function Kernel press}.
\end{align}
\noindent We recognize the term in the second line of equation \eqref{app E: eq: bounded Green's function Kernel press} as the Green's function kernel of the coupled pressure diffusion partial differential equation. This expression has the added advantage that the influence of the thermal load on the pressure $\tilde{p}(x,t)=p(x,t)-p_0$ solution is straightforward. Noticing that for a general diffusion problem on a bounded domain under homogeneous Dirichlet boundary conditions the Green's function kernel is given by:
\begin{align}
G_{X11}(x,x^\prime,t-t^\prime,c) = \frac{2}{\text{H}}\sum_{n=1}^{\infty}\exp{\left[-\lambda^2_nc\frac{t-t^\prime}{\text{H}^2}\right]}\sin{\lambda_n x}\sin{\lambda_n x^\prime}.
\end{align}
The Green's function kernel of the coupled pressure differential equation on the bounded domain is then given as:
\begin{align}
G_{X11}(x,x^\prime,t-t^\prime,c_{th},c_{hy}) =\frac{ c_{hy}G_{X11}(x,x^\prime,t-t^\prime,c_{hy})-c_{th}G_{X11}(x,x^\prime,t-t^\prime,c_{th})}{c_{hy}-c_{th}}.
\end{align}
\noindent Finally, the pressure solution can be given as:
\begin{align}
p(x,t)-p_0=\tilde{p}(x,t)=\frac{\Lambda}{\rho C}\int_0^t\int_{-\infty}^\infty g(x^\prime,t^\prime)G_{X11}(x,x^\prime,t-t^\prime,c_{th},c_{hy})dx^\prime dt^\prime
\end{align}
This result agrees with the formula provided in \cite{Lee1987,Rice2006} for the unbounded domain.
\subsection{Moving thermal load, coupled pore fluid pressure Green's kernel for a unbounded domain.}
\noindent Here, we present the derivation of the Green's function kernel of the coupled pressure diffusion equation for an unbounded domain under moving thermal load. Note here, that the Green's function kernel is independent of the type of loading (stationary or moving), it depends on the kind of the differential operator and the boundary conditions. What differs here in the form of the Green's function kernel is the velocity dependence, since we want to connect the pressure evolution not with the stationary Green's function but with  the moving Dirac thermal load, that can be written as $g(x,t)=\frac{\dot{\delta}}{\rho C}\tau(t)\delta(x-vt)$. In essence we need to only prescribe the velocity dependence of $x^\prime=f(v,t^\prime)$ in the Green's function kernel for the unbounded domain under Dirichlet conditions $G_{X00}(x,x^\prime,(t-t^\prime),c_{hy},c_{th})$. We provide a full description and then compare the results. The coupled system of temperature and pore fluid pressure diffusion equations in the unbounded domain is given by:
\begin{align}
&\frac{\partial T(x,t)}{\partial t}-c_{th}\frac{\partial^2 T(x,t)}{\partial x^2}=\frac{\dot{\delta}}{\rho C}\tau(t)\delta(x-vt),\;-\infty<x<\infty,\;0<t<\infty\nonumber\\
&\frac{\partial \tilde{p}(x,t)}{\partial t}-c_{hy}\frac{\partial^2 \tilde{p}(x,t)}{\partial x^2}=\Lambda\frac{\partial T(x,t)}{\partial t},\;-\infty<x<\infty,\;0<t<\infty,\nonumber\\
&T(x,0)=0,\nonumber\\
&\lim{T(x,t)}\|_{x=-\infty,x=\infty}=0,\nonumber\\
&\tilde{p}(x,0)=0,\nonumber\\
&\lim{\tilde{p}(x,t)}\|_{x=-\infty,x=\infty}=0 \label{app E: eq: system_of_pdes}
\end{align}
\noindent To account for the moving load we perform a change of variables on the original system \eqref{app E: eq: system_of_pdes} where $\xi=x-vt,\;\eta=t$ so that we attach a frame of reference to the moving load. In this case and by suitable application of the chain rule we can write:
\begin{align}
&\frac{\partial T(\xi,\eta)}{\partial \eta}-v\frac{\partial T}{\partial \xi}-c_{th}\frac{\partial^2 T(\xi,\eta)}{\partial \xi^2}=\frac{1}{\rho C}\tau(t)\delta(\xi),\;-\infty<\xi<\infty,\;0<\eta<\infty,\nonumber\\
&\frac{\partial \tilde{p}(\xi,\eta)}{\partial eta}-v\frac{\partial \tilde{p}(\xi,\eta)}{\partial \xi}-c_{hy}\frac{\partial^2 \tilde{p}(\xi,\eta)}{\partial \xi^2}=\Lambda\frac{\partial T(\xi,\eta)}{\partial \eta},\;-\infty<\xi<\infty,\;0<\eta<\infty\nonumber\\
&T(\xi,0)=0,\nonumber\\
&\lim{T(\xi,\eta)}\|_{\xi=-\infty,\xi=\infty}=0,\nonumber\\
&\tilde{p}(\xi,0)=0,\nonumber\\
&\lim{\tilde{p}(\xi,\eta)}\|_{\xi=-\infty,\xi=\infty}=0 \label{app E: eq: system_of_pdes_mov}
\end{align}
\noindent Applying a Fourier transform in space and a Laplace transform in time on the system of partial differential equations \eqref{app E: eq: system_of_pdes_mov} we obtain:
\begin{align}
&s T(k,s)-v(ik)T(k,s)-c_{th}(ik)^2T(k,s)=\frac{1}{\rho C}\tau(s),\nonumber\\
&s \tilde{P}(k,s)-v(ik)\tilde{P}(k,s)-c_{th}(ik)^2\tilde{P}(k,s)=\Lambda s T(k,s).\label{app E: eq: system_of_trans}
\end{align}
\noindent Solving the above algebraic system \eqref{app E: eq: system_of_trans} we obtain:
\begin{align}
&T(k,s) = \frac{1}{\rho C}\frac{\tau{(s)}}{s-v(ik)+c_{th}k^2},\\
&\tilde{P}(k,s) = \frac{\Lambda\tau(s)}{\rho C}\frac{s}{(s-v(ik)+c_{th}k^2)(s-v(ik)+c_{hy}k^2)}
\end{align}
\noindent Inverting the Laplace and then the Fourier transform yields:
\begin{align}
&T(x,t)= \frac{\dot{\delta}}{\rho C }\int_0^t\frac{\tau(t^\prime)}{2\sqrt{\pi c_{th}(t-t^\prime)}}\exp{\left[-\frac{(x-vt^\prime)^2}{4 c_{th}(t-t^\prime)}\right]} dt^\prime,\\
&\begin{aligned}
\tilde{p}(x,t)= \frac{\Lambda\dot{\delta}}{\rho C (c_{hy}-c_{th})}\int_0^t&\frac{\tau(t^\prime)}{2\sqrt{\pi(t-t^\prime)}}\left(\sqrt{c_{hy}}\exp{\left[-\frac{(x-vt^\prime)^2}{4 c_{hy}(t-t^\prime)}\right]} -\sqrt{c_{th}}\exp{\left[-\frac{(x-vt^\prime)^2}{4 c_{th}(t-t^\prime)}\right]} \right)\nonumber\\
&dt^\prime.
\end{aligned}
\end{align}
\noindent  By inspection we note that these are the same expressions as the ones presented in \eqref{ch: 6 eq: G_X00_kernel}, where $x^\prime $ was replaced by $x^\prime=v t^\prime$ and $c=c_{th},\;\text{or}\;c=c_{hy}$ respectively.
%\nocite{*} 
\typeout{}
