# Supplementary material for: Fault friction under thermal pressurization during large coseismic-slip Part I: Numerical analyses
Source: arXiv:2205.00314 source file (2022-04-30)
Supplement: Supplementary file 2 [file AppendixF.tex]

%\chapter{Appendix F \label{Appendix F}}
\section{Frictional behavior for a traveling thermal load on a bounded domain.\label{Appendix F}}
\noindent We continue our analysis by applying a traveling instability on the bounded domain. Again we assume that the traveling plastic strain localization is wholly contained on a mathematical plane moving with a velocity $v$. The plastic strain rate is allowed to travel inside the plastified region of the layer $h$. We note that the plastified region $h$ does not contain the whole layer. This is also the case in the non linear analyses of chapter \ref{ch: 5}, where due to the influence of the layer's boundary conditions the plastified region is smaller than the fault gouge thickness. The integral equation for the determination of the fault's frictional behavior in this case is given by:
\begin{align}
\tau(t) &= f (\sigma_n - p_0) - \frac{f\Lambda\dot{\delta}}{\rho C (c_{hy}-c_{th})}\int_0^t\tau(t^\prime)G_{X11}(x, vt^\prime,t-t^\prime,c_{th},c_{hy}))\big{\|}_{x=0.5L} dt^\prime,
\label{ch: 6 eq: tau_bounded_mov_init}
\end{align}
\noindent where,
\begin{align}
&\begin{aligned}
G_{X11}(x, vt^\prime,t-t^\prime,c_{th},c_{hy}) &= \sum_{m=1}^{\infty}c_{hy}\exp{\left[-m^2\pi^2c_{hy}\frac{t-t^\prime}{\text{H}^2}\right]}\sin{\left(m\pi\frac{vt}{\text{H}}\right)}\sin{\left(m\pi\frac{vt^\prime}{\text{H}}\right)}\\
&\;-\sum_{m=1}^{\infty}c_{th}\exp{\left[-m^2\pi^2c_{th}\frac{t-t^\prime}{\text{H}^2}\right]}\sin{\left(m\pi\frac{vt}{\text{H}}\right)}\sin{\left(m\pi\frac{vt^\prime}{\text{H}}\right)}.
\end{aligned}
\end{align}
\noindent We rewrite equation \eqref{ch: 6 eq: tau_bounded_mov_init} with the help of $\alpha_m=\frac{m\pi v}{\text{H}}$, replacing the $\sin\left(\alpha_m t\right)$,$\sin\left(\alpha_m t^\prime\right)$ terms, with the help of the exponential trigonometric identity, $\sin{\omega}=\frac{\exp{(i \omega)}-\exp{(-i \omega)}}{2i}$, distributing the exponentials we arrive at:
\begin{align}
&\begin{aligned}
\tau(t) &= f (\sigma_n - p_0)\\
& - \frac{ f\Lambda\dot{\delta}}{2\text{H} \rho C (c_{hy}-c_{th})}\int_0^t\tau(t^\prime)\sum_{m=1}^{\infty}K(v,t-t^\prime,m)\exp{(i \alpha_m( t+ t^\prime))} dt^\prime\\
&- \frac{ f\Lambda\dot{\delta}}{2\text{H} \rho C (c_{hy}-c_{th})}\int_0^t\tau(t^\prime)\sum_{m=1}^{\infty}K(v,t-t^\prime,m)\exp{(-i \alpha_m( t+ t^\prime))} dt^\prime\\
&- \frac{f \Lambda\dot{\delta}}{2\text{H} \rho C (c_{hy}-c_{th})}\int_0^t\tau(t^\prime)\sum_{m=1}^{\infty}K(v,t-t^\prime,m)\exp{(i \alpha_m( t- t^\prime))}dt^\prime\\
&- \frac{ f\Lambda\dot{\delta}}{2\text{H} \rho C (c_{hy}-c_{th})}\int_0^t\tau(t^\prime)\sum_{m=1}^{\infty}K(v,t-t^\prime,m)\exp{(-i \alpha_m( t- t^\prime))} dt^\prime.
\end{aligned}
\end{align}
\noindent where $K(v,t,m)=c_{hy}\exp{\left[-\frac{\alpha^2_mc_{hy}}{v^2}(t)\right]}-c_{th}\exp{\left[-\frac{\alpha^2_mc_{th}}{v^2}(t-t^\prime)\right]}$, we note here that $t+t^\prime$ can be expressed as $2t -(t-t^\prime)$, making use of the exponential identities the above expression can be written as:
\begin{align}
&\begin{aligned}
\tau(t) &= f (\sigma_n - p_0)\\
& - \sum_{m=1}^{\infty}\frac{f\Lambda\dot{\delta} \exp{(2i \alpha_m t)}}{2\text{H} \rho C (c_{hy}-c_{th})}\int_0^t\sum_{m=1}^{\infty}\tau(t^\prime)K_1(v,t-t^\prime,m) dt^\prime\\
& - \sum_{m=1}^{\infty}\frac{f\Lambda\dot{\delta} \exp{(-2i \alpha_m t)}}{2\text{H} \rho C (c_{hy}-c_{th})}\int_0^t\sum_{m=1}^{\infty}\tau(t^\prime)K_2(v,t-t^\prime,m) dt^\prime\\
& - \sum_{m=1}^{\infty}\frac{f\Lambda\dot{\delta} }{2\text{H} \rho C (c_{hy}-c_{th})}\int_0^t\sum_{m=1}^{\infty}\tau(t^\prime)c_{hy}K_1(v,t-t^\prime,m) dt^\prime\\
& - \sum_{m=1}^{\infty}\frac{f\Lambda\dot{\delta} }{2\text{H} \rho C (c_{hy}-c_{th})}\int_0^t\sum_{m=1}^{\infty}\tau(t^\prime)c_{hy}K_2(v,t-t^\prime,m) dt^\prime,\\
\end{aligned}\label{ch: 6 eq: intgral_trav_bounded_f1}
\end{align}
\noindent where:
\begin{align}
K_1(v,t,m)=c_{hy}\exp{\left[-\left(\frac{\alpha^2_mc_{hy}}{v^2}+i\alpha_m\right)(t)\right]}-c_{th}\exp{\left[-\left(\frac{\alpha^2_mc_{th}}{v^2}+i\alpha_m\right)(t)\right]},\nonumber\\
K_2(v,t,m)=c_{hy}\exp{\left[-\left(\frac{\alpha^2_mc_{hy}}{v^2}-i\alpha_m\right)(t)\right]}-c_{th}\exp{\left[-\left(\frac{\alpha^2_mc_{th}}{v^2}-i\alpha_m\right)(t)\right]}.
\end{align}
\noindent  Now every term in the above summations corresponds to a convolution integral and the modified CQM $\mathcal{Z}$-Transform method can be applied. In contrast to previous cases we note that the first two summation terms contain an exponential term to an imaginary power ($\exp{2i\alpha_m t}$) that indicates an oscillation in time.\\ %The application of the the modified CQM $\mathcal{Z}$-Transform method in this case is developed in the Appendix \ref{Appendix E}. We will not pursue this further however, since this solution procedure becomes more involved and it lies outside the scope of this Thesis. Furthermore, the traveling shear band of chapter \ref{ch: 5} travels inside the plastified region $h$ in a periodic fashion.\\ %The results of the above approach can be compared to the Adomian Decomposition Method (ADM), a standard procedure for solving integral equations \cite{wazwaz2011linear}.
\newline
\noindent The convolution integrals defined in equation \eqref{ch: 6 eq: intgral_trav_bounded_f1} require a special handling  during the application of the CQM method. We start for equation \eqref{ch: 6 eq: intgral_trav_bounded_f1}. We start by rewriting the kernel with the help of its inverse Laplace transform. 
\begin{align}
&\begin{aligned}
\tau(t) &= f (\sigma_n - p_0)\\
& -\frac{f\Lambda\dot{\delta}}{4L \rho C \pi i} \sum_{m=1}^{\infty}\int_{\gamma-i\infty}^{\gamma+i\infty}\int_0^t\tau(t^\prime)G^1_{X11}(s,m)\exp{\left[-s(t-t^\prime)+i \alpha_m 2t\right]}dt^\prime ds \\
& -\frac{f\Lambda\dot{\delta}}{4L \rho C \pi i} \sum_{m=1}^{\infty}\int_{\gamma-i\infty}^{\gamma+i\infty}\int_0^t\tau(t^\prime)G^2_{X11}(s,m)\exp{\left[-s(t-t^\prime)-i \alpha_m 2t\right]}dt^\prime ds \\
& -\frac{f\Lambda\dot{\delta}}{4L \rho C \pi i} \sum_{m=1}^{\infty}\int_{\gamma-i\infty}^{\gamma+i\infty}\int_0^t\tau(t^\prime)G^1_{X11}(s,m)\exp{\left[-s(t-t^\prime)\right]}dt^\prime ds \\
& -\frac{f\Lambda\dot{\delta}}{4L \rho C \pi i} \sum_{m=1}^{\infty}\int_{\gamma-i\infty}^{\gamma+i\infty}\int_0^t\tau(t^\prime)G^2_{X11}(s,m)\exp{\left[-s(t-t^\prime)\right]}dt^\prime ds \\
\end{aligned}\label{app F: eq: intgral_trav_bounded_app1}
\intertext{where $G^1_{X11}(s,m),G^2_{X11}(s,m),G^3_{X11}(s,m),G^4_{X11}(s,m)$ are given by:}
&G^1_{X11}(s,m)=\frac{1}{c_{hy-c_{th}}}\left(c_{hy}\frac{1}{s+\left(\frac{\alpha_m^2c_{hy}}{v^2}+i\alpha_m\right)}-c_{th}\frac{1}{s+\left(\frac{\alpha_m^2c_{th}}{v^2}+i\alpha_m\right)}\right),\\
&G^2_{X11}(s,m)=\frac{1}{c_{hy-c_{th}}}\left(c_{hy}\frac{1}{s+\left(\frac{\alpha_m^2c_{hy}}{v^2}-i\alpha_m\right)}-c_{th}\frac{1}{s+\left(\frac{\alpha_m^2c_{th}}{v^2}-i\alpha_m\right)}\right).
%,\\
%&G^3_{X11}(s,m)=\frac{1}{c_{hy-c_{th}}}\left(c_{hy}\frac{1}{s+\left(\frac{\alpha_m^2c_{hy}}{v^2}+i\alpha_m\right)}-c_{th}\frac{1}
%{s+\left(\frac{\alpha_m^2c_{th}}{v^2}+i\alpha_m\right)}\right),\\
%&G^4_{X11}(s,m)=\frac{1}{c_{hy-c_{th}}}\left(c_{hy}\frac{1}{s+\left(\frac{\alpha_m^2c_{hy}}{v^2}-i\alpha_m\right)}-c_{th}\frac{1}
%{s+\left(\frac{\alpha_m^2c_{th}}{v^2}-i\alpha_m\right)}\right).
\end{align}
\noindent Here, for the first two terms in equation \eqref{app F: eq: intgral_trav_bounded_app1}, we make the observation that the integrals involving the quantities of $(t-t^\prime), t^\prime$ are solutions to the first order linear differential equations:
\begin{align}
&\frac{d h_{1m}(t)}{dt}=(s+2\alpha_m i )h_{1m}(t)+\tau(t)\exp{\left[-2\alpha_m i t\right]},\; h_1(0)=0,\; t\geq 0,\label{app F: eq: h1_aux_prob}\\
&\frac{d h_{2m}(t)}{dt}=(s-2\alpha_m i )h_{2m}(t)+\tau(t)\exp{\left[2\alpha_m i t\right]},\; h_2(0)=0,\; t\geq 0,\label{app F: eq: h2_aux_prob}
\end{align}
\noindent while the integrals in the last two terms are solutions to the first order linear differential equation \eqref{ch: 6 eq: aux_diff_equation}. We apply next the $\mathcal{Z}$-Transform to the sampled linear integral equation \eqref{app F: eq: intgral_trav_bounded_app1}. 
\begin{align}
&\begin{aligned}
T(z) = f (\sigma_n - p_0)\frac{z}{z-1}-\frac{f\Lambda\dot{\delta}}{4L \rho C \pi i}\left( \sum_{m=1}^{\infty} \right.& \int_{\gamma-i\infty}^{\gamma+i\infty}G^1_{X11}(s,m)H_1(z,m) ds\nonumber\\
&+ \int_{\gamma-i\infty}^{\gamma+i\infty}G^2_{X11}(s,m)H_2(z,m)ds\\
&+ \int_{\gamma-i\infty}^{\gamma+i\infty}G^1_{X11}(s,m)H(z,m) ds\nonumber\\
&\left.  +\int_{\gamma-i\infty}^{\gamma+i\infty})G^2_{X11}(s,m)H(z,m)ds\right) \\
\end{aligned}\label{app F: eq: intgral_trav_bounded_trans}
\end{align}
\noindent To evaluate $T(z)$ we need the expressions of $H_1(z,m),H_2(z,m),H(z,m)$ as functions of $T(z)$. While the expression for $H(z,m)$ remains the same as the one derived in the main text (see equation \eqref{ch: 6 eq: discretized aux problem}), the sampled differential equations  \eqref{app F: eq: h1_aux_prob},\eqref{app F: eq: h2_aux_prob} at points $t_n=n\Delta t$ are transformed with the help of the $\mathcal{Z}$-Transform properties to:
\begin{align}
&\frac{z-1}{z\Delta t}H_1(z,m) = (s+2\alpha_m \Delta t \;i)H_1(z,m)+T(\frac{z}{\exp{\left[2 \alpha_m \Delta t\; i\right]}}),\\
&\frac{z-1}{z\Delta t}H_2(z,m) = (s-2\alpha_m \Delta t\; i)H_2(z,m)+T(\frac{z}{\exp{\left[-2 \alpha_m \Delta t\; i\right]}}).
\end{align}
\noindent The transformed auxiliary functions are given as:
\begin{align}
&H_1(z,m) =\frac{T(\frac{z}{\exp{\left[2 \alpha_m \Delta t\;i\right]}})}{\frac{z-1}{z\Delta t}- (s+2\alpha_m \Delta t \; i)},\\
&H_2(z,m) =\frac{T(\frac{z}{\exp{\left[-2 \alpha_m \Delta t\; i\right]}})}{\frac{z-1}{z\Delta t}- (s-2\alpha_m \Delta t\;i)}.
\end{align}
\noindent Applying then into equation \eqref{app F: eq: intgral_trav_bounded_trans} we obtain:
\begin{align}
&\begin{aligned}
T(z) &= f (\sigma_n - p_0)\frac{z}{z-1}
-\frac{f\Lambda\dot{\delta}}{4L \rho C \pi i}\sum_{m=1}^{\infty}\left(\int_{\gamma-i\infty}^{\gamma+i\infty}G^1_{X11}(s,m)\frac{T(\frac{z}{\exp{\left[2 \alpha_m \Delta t \; i\right]}})}{\frac{z-1}{z\Delta t}- (s+2\alpha_m \Delta t \; i)} ds\right.\\
&+\int_{\gamma-i\infty}^{\gamma+i\infty}G^2_{X11}(s,m)\frac{T(\frac{z}{\exp{\left[-2 \alpha_m \Delta t \; i\right]}})}{\frac{z-1}{z\Delta t}- (s-2\alpha_m \Delta t \; i)}ds +\int_{\gamma-i\infty}^{\gamma+i\infty}G^1_{X11}(s,m)\frac{T(z)}{\frac{z-1}{z\Delta t}- s} ds\\
& \left.+ \int_{\gamma-i\infty}^{\gamma+i\infty}G^2_{X11}(s,m)\frac{T(z)}{\frac{z-1}{z\Delta t}- s}ds \right).\label{app F: eq: intgral_trav_bounded_trans2}
\end{aligned}
\end{align}
\noindent Applying the Cauchy residue theorem of complex analysis on equation \eqref{app F: eq: intgral_trav_bounded_trans2} we get:
\begin{align}
&\begin{aligned}
T(z) &= f (\sigma_n - p_0)\frac{z}{z-1}
-\frac{f\Lambda\dot{\delta}}{2\text{H} \rho C }\sum_{m=1}^{\infty}\left(G^1_{X11}\left(\frac{z-1}{z\Delta t}-2\alpha_m \Delta t \; i\right)T\left(\frac{z}{\exp{\left[2 \alpha_m \Delta t \; i\right]}}\right)\right.\\
&+G^2_{X11}\left(\frac{z-1}{z\Delta t}+2\alpha_m \Delta t \;  i\right)T\left(\frac{z}{\exp{\left[-2 \alpha_m \Delta t \; i\right]}}\right) +G^3_{X11}\left(\frac{z-1}{z\Delta t}\right)T(z)\nonumber\\
&\left.+G^4_{X11}\left(\frac{z-1}{z\Delta t}\right)T(z) \right).
\label{app F: eq: final_functional_equation}
\end{aligned}
\end{align}
\noindent Contrary to the previous cases examined in the main text, in this case the equation obtained is a functional equation, and the problem is not simplified. We make the following observations:
\begin{itemize}
\item[•]According to the value of $\alpha_m = \frac{m \pi v}{\text{H}}$ we note that the denominators of the functional terms lie on the unit circle of the complex $z$ plane. This is a very important information since for finding the inverse of the transformation we need to integrate along a closed contour containing the origin. To simplify our calculations we can take the contour to be a concentric circle to the unit circle in the z plane under the term that we include all the poles of $T(z)$. We can then evaluate the integral by calculating the values of the functional expression at points coincident to the scaled unit circle points used in the expression definition.
\item[•] It is always the kernel that controls the poles and branch cuts of $T(z)$, the kernel in this case has not changed from the one used in the bounded case, therefore the same circle with radius of integration 1.1 is valid for the purposes of our analysis. 
\item[•] By letting $m$ increase, eventually we arrive at repeated values of the denominators in $T(\frac{z}{\exp{2\alpha_m i}}), T(\frac{z}{\exp{-2\alpha_m i}}) $. Because the transform has an inverse, the values of  $T(\frac{z}{\exp{2\alpha_m i}}), T(\frac{z}{\exp{-2\alpha_m i}}) $ have to lie on the same Riemann sheet. Moreover, our kernel presented no branch cuts therefore, we don't need to account for the possibility of double values of $T$.
\item[•] As we apply the values around the unit circle increasing $m$ on the above functional expression, we see that we get extra $m+k,m-k$ terms due to the form of the equation. We note that according to the previous observations, they can safely be neglected since the values on the unit circle constitute a $k\times{}k$ system of independent unknowns and equations whose determinant is non zero.
\item[•] Generalizing even more we can treat each of the different $T(\frac{z}{\exp{2\alpha_m i}}), T(\frac{z}{\exp{-2\alpha_m i}}) $ scalings of $T(z)$ as independent functions $T_{i}(z)$. This way of reasoning produces a system of unknown independent functions. By evaluating at the scaled points to the unit circle the functional system reduces to the algebraic system defined above.  
\end{itemize}
\noindent We know that our problem is stable and causal. This means that all of the potential poles of $T(z)$ must lie inside the unit circle, and the region of convergence of $T(z)$ is the whole $z$ complex plain except the region interior to the unit circle. We choose to integrate along a circle centered at the origin of the $z$ plane with radius $R=1.1$ m. We choose to sample the points on the circle every $\Delta t=0.0001$ (s). Based on the observations above, we evaluate the functional equation \eqref{app F: eq: final_functional_equation} at the points along the circle $z=1.1\exp{\left[2\alpha_k \Delta t \; i\right]}=1.1\exp{\left[2k\pi\frac{ v \Delta t}{\text{H}}i\right]}$. We note that when $\left(k\frac{v\Delta t}{\text{H}}\right)$ is a whole number, our selection process will have traveled around the circle one time. For a first pass around the circle we require that $k_{max}=\frac{\text{H}}{v\Delta t}$. Increasing $k$ more than $k_{max}-1$ will result in a repetition of the algebraic equations due to the observations established above.  In this case the algebraic equations that will be produced by substitution to the functional equation \eqref{app F: eq: final_functional_equation} won't be independent. The following system of unknown points is found:
\begin{align}
&\begin{aligned}
&k=0&\\
&\begin{aligned}
T\left(1.1\right) &= f (\sigma_n - p_0)\frac{z}{z-1}\bigg{\|}_{z=1.1}\\
&-\frac{\Lambda\dot{\delta}}{2\text{H} \rho C }\sum_{m=1}^{\infty}\left(G^1_{X11}(z,\beta_m)\bigg{\|}_{z=1.1}\right.
T\left(1.1\exp{\left[(\beta_0-\beta_m) i\right]}\right)\nonumber\\
&+G^2_{X11}(z,\beta_m)\bigg{\|}_{z=1.1}T\left(1.1\exp{\left[(\beta_0+\beta_m)i\right]}\right)\\
&\left.+G^3_{X11}(z,\beta_m)\bigg{\|}_{z=1.1}T(1.1)+G^4_{X11}(z,\beta_m)\bigg{\|}_{z=1.1}T(1.1\exp{\left[\beta_0 i\right]})\right).
\end{aligned}
\end{aligned}
\end{align}
\begin{align}
&\begin{aligned}
&k=1&\\
&\begin{aligned}
T\left(1.1\exp{\left[\beta_1 i\right]}\right) &= f (\sigma_n - p_0)\frac{z}{z-1}\bigg{\|}_{z=1.1}\\
&-\frac{\Lambda\dot{\delta}}{2\text{H} \rho C }\sum_{m=1}^{\infty}\left(G^1_{X11}(z,\beta_m)\bigg{\|}_{z=1.1}\right. T\left(1.1\exp{\left[(\beta_1-\beta_m) i\right]}\right)\nonumber\\
&+G^2_{X11}(z,\beta_m)\bigg{\|}_{z=1.1}T\left(1.1\exp{\left[(\beta_1+\beta_m)i\right]}\right)\\
&+G^3_{X11}(z,\beta_m)\bigg{\|}_{z=1.1}T(1.1\exp{\left[\beta_1 i\right]})\nonumber\\
&\left.+G^4_{X11}(z,\beta_m)\bigg{\|}_{z=1.1}T(1.1\exp{\left[\beta_1 i\right]}) \right).
\end{aligned}
\end{aligned}
\end{align}
\begin{align}
&\begin{aligned}
&k=k_{max}-1&\\
&\begin{aligned}
T\left(1.1\exp{\left[\beta_k\;i\right]}\right) &= f (\sigma_n - p_0)\frac{z}{z-1}\bigg{\|}_{z=1.1\exp{\left[\beta_k\;i\right]}}\\
&-\frac{\Lambda\dot{\delta}}{2\text{H} \rho C }\sum_{m=1}^{\infty}\left(G^1_{X11}(z,\beta_m)\bigg{\|}_{z=1.1\exp{\left[\beta_k\;i\right]}}T\left(1.1\exp{\left[(\beta_k-\beta_m) i\right]}\right)\right.\\
&\left.+G^2_{X11}(z,\beta_m)\bigg{\|}_{z=1.1\exp{\left[\beta_k i\right]}}T\left(1.1\exp{\left[(\beta_k+\beta_m)i\right]}\right)\right.\\
&+G^3_{X11}(z,\beta_m)\bigg{\|}_{z=1.1\exp{\left[\beta_k \;i\right]}}T(1.1\exp{\left[\beta_k i\right]})+G^4_{X11}(z,\beta_m)\bigg{\|}_{z=1.1\exp{\left[\beta_k\;i\right]}}
\end{aligned}\\
&&\left.T(1.1\exp{\left[\beta_k i\right]}) \right).
\end{aligned}
\end{align}
\noindent Where $\beta_m=2m\pi\frac{ v \Delta t}{\text{H}},\;\beta_k=2k\pi\frac{ v \Delta t}{\text{H}}$. We not again that based on our observations that non zero values of T(z) are found when the argument of $z$ lies between $([0,2\pi)) $ which in turn implies that only the values of T(z) whose argument lies between $\beta_k-\beta_m\geq$ and $\beta_k+\beta_m<2\pi$ are taken into account. Having calculated all the values that are important, we are left with a system that can be solved algebraically for their determination. Therefore, calculating the contour integrals for the numerical inversion of the $\mathcal{Z}$-Transform becomes once again possible.\\
\newline
\noindent All this discussion covers only the case, where the strain localization travels to one direction inside the plastified region of the fault gouge. However form chapter \ref{ch: 5} we knot that the strain localization travels periodically inside the plastified region of the fault gouge. We will not pursue this further however, since this solution procedure becomes more involved and it lies outside the scope of this Thesis.\\
\newline
 \noindent Another way of handling the problem is to use the method of the Adomian Decomposition \cite{wazwaz2011linear}. This way the functions needed for the determination of the original unknown are always known based on the previous step of the Adomian method. Since the method is sensitive to the number of terms and the integral calculation we can use the $CQM$ $\mathcal{Z}$-Transform method to handle the successive convolutions. Finally, the collocation method used in chapter \ref{ch: 6} of this thesis is in our opinion the most efficient method of solving the problem when periodic loading paths are studied. 
%\nocite{*} 
%\typeout{}
