# Supplementary material for: Fault friction under thermal pressurization during large coseismic-slip Part I: Numerical analyses
Source: arXiv:2205.00314 source file (2022-04-30)
Supplement: Supplementary file 3 [file AppendixH.tex]

%\chapter{Appendix H \label{Appendix H}}
\section{Collocation Methodology\label{Appendix H}}
\noindent In order to apply the collocation methodology to the linear Volterra integral equation of the second kind in chapter \ref{ch: 6}, \eqref{ch: 6 eq: integral equation1}, we make use of the collocation methodology described in \cite{tang2008spectral}. The integral equation is given as:
\begin{align}
\tau(t) = f(\sigma_n-p_0)-C\int_0^t\tau(t^\prime)G^\star(t-t^\prime,c_{hy},c_{th}) dt^\prime,\; t\in [0,T] \label{app: H eq: integral equation1},
\end{align}
\noindent where $f(\sigma_n-p_0), G^\star(t,c_{th},c_{hy})$ are given functions, and $\tau(t)$ is the unknown function. We begin by performing a change of variables from $t\in [0,T]$ to $x\in [-1,1]$. The change of variables reads:
\begin{align*}
t=T\frac{1+x}{2},\;x=\frac{2t}{T}-1
\end{align*}
\noindent The Volterra integral equation can then be written:
\begin{align}
u(x) = f(\sigma_n-p_0)-C\int_0^{T\frac{1+x}{2}}G^\star(T\frac{1+x}{2}-t^\prime,c_{hy},c_{th})dt^\prime,\; x\in [-1,1] \label{app: H eq: integral equation2},
\end{align} 
\noindent where $u(x)=\tau(T\frac{1+x}{2})$. In order for the collocation method solution to converge exponentially we require that both the integral equation \eqref{app: H eq: integral equation2} and the integral inside \eqref{app: H eq: integral equation2} are expressed inside the same interval $[-1,1]$. To do this first we change the integration bounds from $t^\prime\in[0,T\frac{1+x}{2}]$ to $s\in [-1,x]$.
\begin{align}
u(x) = f(\sigma_n-p_0)-C\int_0^{x}K(x,s,c_{hy},c_{th})ds,\; x\in [-1,1], \label{app: H eq: integral equation3},
\end{align} 
\noindent where $K(x,s)=\frac{T}{2}G^\star\frac{T}{2}(x-s),c_{hy},c_{th})$. Next, we set the $N+1$ collocation points $x_i\in [-1,1]$ and corresponding weights $\omega_i$ according to the Gauss-Legendre quadrature formula. The integral equation \eqref{app: H eq: integral equation3} must hold at each $x_i$:
\begin{align}
u(x_i) = f(\sigma_n-p_0)-C\int_0^{x_i}K(x_i,s,c_{hy},c_{th})ds,\; i\in [0,N], \label{app: H eq: integral equation4},
\end{align}
\noindent The main hindrance in solving equation \eqref{app: H eq: integral equation4} accurately, is the calculation of the integral with variable integration bounds. For small values of $x_i$, the quadrature provides little information for $u(s)$. We handle this difficulty by yet another variable change where we transfer the integration variable $s\in [-1,x_i]$ to $\theta\in [-1,1]$ via the transformation:
\begin{align}
s(x,\theta)=\frac{1+x}{2}\theta+\frac{x-1}{2},\;\theta \in [-1,1].
\end{align}
Thus, equation \eqref{app: H eq: integral equation4} is transformed into:
\begin{align}
u_i+\frac{1+x_i}{2}\sum\limits_{j=0}^Nu_j\sum\limits_{p=0}^N K(x_i,s(x_i,\theta))u(s(x_i,\theta_p))\omega_j=f(\sigma_n-p_0),\; i\in [0,N]
\end{align}
\noindent In order to apply the collocation method according to the Gauss Legendre quadrature we express the solution $u(s(x_i,\theta_j))$ with the help of Lagrange interpolation polynomials $F_j(s(x_i,\theta_j))$ as a series: $u(s(x_i,\theta_j)) \sim \sum  \limits_{k=0}^N u_jF_j(s(x_i,\theta_j))$
\begin{align}
u_i+\frac{1+x_i}{2}\sum\limits_{j=0}^Nu_j\left(\sum\limits_{p=0}^N K(x_i,s(x_i,\theta))F_j(s(x_i,\theta_p))\omega_p\right)=f(\sigma_n-p_0),\; i\in [0,N].
\end{align}
\noindent In order to assure an exponential degree of convergence we choose that the set of Gauss-Legendre quadrature points for the numerical evaluation of the integral $\{\theta_j\}_{j=0}^N$ coincides with the set of collocation points $\{x_j\}$, where the integral equation is evaluated. Rearranging the terms and applying Einstein's summation over repeated indices yields the system of algebraic equations:
\begin{align}
(\delta_{ij}+A_{ij})u_j=g(x_i),
\end{align}
\noindent where, $A_{ij} =\frac{1+x_i}{2}\sum\limits_{j=0}^N\left(\sum\limits_{p=0}^N K(x_i,s(x_i,\theta))F_j(s(x_i,\theta_p))\omega_p\right),\; g(x_i)=f(\sigma_n-p_0)$ and $u_j$ the unknown quantities. Since the Gauss-Lagrange quadrature was assumed the interpolation coefficients $u_j$ calculated at each $x_j$ are also the value of the interpolation at $x_j$.
