# Supplementary material for: Fault friction under thermal pressurization during large coseismic-slip Part I: Numerical analyses
Source: arXiv:2205.00314 source file (2022-04-30)
Supplement: Supplementary file 4 [file AppendixI.tex]

%\chapter{Appendix I \label{Appendix I}}
\section{Proof that the maximum of pressure and the position of the yielding plane (thermal load) coincide \label{Appendix I}}
\noindent In this appendix we will present the central part of our argument in chapter \ref{ch: 6} concerning the applicability of a traveling strain localization mode. I chapter \ref{ch: 6} we have argued that in order for the strain localization mode to be applicable to the problem at hand it needs to satisfy the equations of equilibrium and it should warrant that the prescribed localization motion corresponding to the position of the yielding plane inside the layer satisfies also the condition that it coincides with the maximum of the pressure profile inside the layer at all times \cite[see][]{Rice2006}.\\
\subsection{Proof of pressure Maxima for the traveling strain localization on an bounded domain.\label{app I: sec: 1}}

\noindent To this end, provided that the function we search for is sufficiently smooth except maybe at a finite number of points, we make use of our tools from calculus that indicate the use of the first and second order derivatives to decide upon the position and the kind of the extremalities of the unknown function. We start our discussion with the case of a traveling localization on a bounded mathematical domain. In this case the derived kernel of the coupled pressure temperature diffusion equation is bounded and smooth at all times $t\in[0,\infty)$. The pressure profile at all times $t$, for a traveling strain localization mode $\dot{\gamma(x,t)}=\dot{\delta}\delta_{Dirac}(x-vt)$ (and thermal load $\frac{1}{\rho C}\tau{t}\dot{\delta}\delta_{Dirac}(x-vt)$) at position $x=vt$  is given by the relation:
\begin{align}
p(x,t)-p_0 =& \frac{2\Lambda \dot{\delta}}{\text{H}\rho C(c_{hy}-c_{th})}\int_0^t\tau(t^\prime)\sum\limits_{m=0}^{\infty}  K(x,t,t^\prime,m)dt^\prime \label{app I: eq: pressure}
\end{align}
\noindent where $K(x,t,t^\prime,m)=
\left(c_{hy}\exp{\left(-m^2\pi^2c_{hy}\frac{t-t^\prime}{\text{H}^2}\right)}-c_{th}
\exp{\left(-m^2\pi^2c_{th}\frac{t-t^\prime}{\text{H}^2}\right)}\right)\sin{\left(m\pi\frac{x}{\text{H}}\right)}\sin{\left(m\pi\frac{vt^\prime}{\text{H}}\right)})$. The first derivative of equation \eqref{app I: eq: pressure} is given by:
\begin{align}
\frac{\partial p(x,t)}{\partial x} =\frac{2\Lambda \dot{\delta} m \pi}{\text{H}^2\rho C(c_{hy}-c_{th})}\int_0^t\tau(t^\prime)\sum\limits_{m=0}^\infty\frac{\partial K(x,t,t^\prime,m)}{\partial x}dt^\prime
\end{align}
\noindent where $\frac{\partial K(x,t,t^\prime,m)}{\partial x}=\left(c_{hy}\exp{\left(-m^2\pi^2c_{hy}\frac{t-t^\prime}{\text{H}^2}\right)}
-c_{th}\exp{\left(-m^2\pi^2c_{th}\frac{t-t^\prime}{\text{H}^2}\right)}\right)\cos{\left(m\pi\frac{x}{\text{H}}\right)}\sin{\left(m\pi\frac{vt^\prime}{\text{H}}\right)}$. We note that for $\frac{\partial p}{\partial x}=0$ we need to find $x$ such that: 
\begin{align}
\Pi(x,t^\prime,m) = \cos{\left(m\pi\frac{x}{\text{H}}\right)}\sin{\left(m\pi\frac{vt^\prime}{\text{H}}\right)}=0.
\end{align} 
\noindent We write the above product with the help of the exponential function.
\begin{align}
\Pi(x,t^\prime,m) &= \frac{\exp{im\pi\frac{x}{\text{H}}}+\exp{-im\pi}\frac{x}{\text{H}}}{2}\frac{\exp{im\pi\frac{vt^\prime}{\text{H}}}-\exp{-im\pi}\frac{vt^\prime}{\text{H}}}{2i}=0,\\
\Pi(x,t^\prime,m) &=\frac{1}{4i}\left(\exp{\left(im\pi\frac{x+vt^\prime}{\text{H}}\right)}+\right.
\left.\exp{\left(-im\pi\frac{x-vt^\prime}{\text{H}}\right)}\right.\nonumber\\
&\left.-\exp{\left(im\pi\frac{x-vt^\prime}{\text{H}}\right)}-\exp{\left(-im\pi\frac{x+vt^\prime}{\text{H}}\right)}\right)=0.
\end{align} 
\noindent Transforming again the above summation with the help of the Euler relations into $\sin{(\cdot{})}+i\cos{(\cdot{})}$ and using the trigonometric equalities between the arguments of the opposite sign we arrive at:
\begin{align}
\frac{1}{2}\sin{\left(m\pi\frac{x-vt^\prime}{\text{H}}\right)}=0,
\end{align}
\noindent which is true $\forall t\in[0,\infty)$ only when $x=vt^\prime$. Thus we know that $p(x,t)-p_0$ presents an extremum an the position of the traveling yielding plane. We need to prove that this extremum is also maximum for every $t>0$. For this we take the second derivative of equation \eqref{app I: eq: pressure}.
\begin{align}
\frac{\partial^2 p(x,t)}{\partial x^2} =\frac{2\Lambda \dot{\delta} m^2 \pi^2}{\text{H}^3\rho C(c_{hy}-c_{th})}\int_0^t\tau(t^\prime)\sum\limits_{m=0}^\infty\frac{\partial^2 K(x,t,t^\prime,m)}{\partial x^2}dt^\prime,\label{app I: eq: pressure sec_der}
\end{align}
\noindent where $\frac{\partial^2 K(x,t,t^\prime,m)}{\partial x^2}=-\left(c_{hy}\exp{\left(-m^2\pi^2c_{hy}\frac{t-t^\prime}{\text{H}^2}\right)}
-c_{th}\exp{\left(-m^2\pi^2c_{th}\frac{t-t^\prime}{\text{H}^2}\right)}\right)\sin{\left(m\pi\frac{x}{\text{H}}\right)}\sin{\left(m\pi\frac{vt^\prime}{\text{H}}\right)}$. Evaluating the second derivative in equation \eqref{app I: eq: pressure sec_der} with respect to $x$ at the position $x=vt^\prime\;\frac{\partial^2 p(x,t) }{\partial x^2}\big{\|}_{x=vt^\prime}$  we see that for $t>0$ equation \eqref{app I: eq: pressure sec_der} is always negative. This means that the extremum at $x=vt^\prime$ is also a maximum. 
\subsection{Proof of pressure Maxima for the traveling strain localization on an unbounded domain. \label{app I: sec: 2}}
\noindent In the case of the unbounded domain due to the form of the coupled temperature and pressure kernel, $G_{T,P}(x,t-t^\prime,c_{th},c_{hy})$, \cite[see][]{Lee1987} resulting in a weakly singular convolution integral, such a derivation is not trivial. While we can ensure the convergence of the integral in a Riemann sense for the original integral and verify the position of its extremalities we cannot directly calculate its second derivative since the resulting integral corresponds to a hyper singular divergent integral. To answer questions about its convergence we need to apply the notion of Hadamard regularization.\\
\newline
\noindent We notice, however, that this question is a special case of the pressure maxima of a traveling strain localization on a bounded domain of height $\text{H}$, when $\text{H}$ tends to $\infty$, see section \ref{app I: sec: 1}.
